# Supplementary material for: Computational and Experimental Investigation of Chiral and Achiral 2D Organic Lead Bromide Perovskites: Octahedral Distortions and Electronic and Optical Properties
Source: arXiv:2509.07152 ancillary file (2025-09-08)
Supplement: Supplementary file 1 [file Supplementary_Information.pdf]

# Supplementary Information: Computational and Experimental Investigation of Chiral and Achiral 2D Organic Lead Bromide Perovskites: Octahedral Distortions and Electronic and Optical Properties

Md Mehdi Masud,<sup>[a]</sup> Jarek Viera,<sup>[b]</sup> Azza Ben-Akacha,<sup>[b]</sup> Biwu Ma,<sup>\*,[b]</sup> David A. Strubbe<sup>\*,[a]</sup>

[a] Md Mehdi Masud, David A. Strubbe  
Department of Physics  
University of California, Merced  
Merced, California 95343, USA  
E-mail: dstrubbe@ucmerced.edu

[b] Jarek Viera, Azza Ben-Akacha, Biwu Ma  
Department of Chemistry and Biochemistry  
Florida State University  
Tallahassee, Florida 32306, USA  
E-mail: bma@fsu.edu

## Synthesis

Synthesis of (R-FMBA)<sub>2</sub>PbBr<sub>4</sub> and (S-FMBA)<sub>2</sub>PbBr<sub>4</sub> crystals were obtained by reacting lead oxide and S-/R-FMBA, in a 1:2 stoichiometric ratio, in 6 mL of hydrobromic acid solution. The prepared solutions were then digested at 100°C with 420 rpm for an hour until they became clear solutions and all reagents were dissolved. Then the vials were opened and left to cool down to room temperature at a natural cooling rate. Plate-like transparent crystals were obtained overnight. Crystals were washed with diethyl ether, dried under vacuum, and stored for further use.

Synthesis of (FBA)<sub>2</sub>PbBr<sub>4</sub> crystals were prepared by dissolving lead oxide and the 4-fluorobenzylamine solution in a 1:1 ratio in a 6 mL hydrobromic acid solution. The solution was then digested at 100°C with 420 rpm for an hour until they became clear solutions and all reagents were dissolved. Then the vial was opened and left to cool down to room temperature at a natural cooling rate. Plate-like transparent crystals were obtained overnight, washed with diethyl ether, dried under vacuum and stored for further use.

Thin films preparation of (R-FMBA)<sub>2</sub>PbBr<sub>4</sub>, (S-FMBA)<sub>2</sub>PbBr<sub>4</sub> 0.2 g/mL DMF solution of dissolved crystals were spin coated on glass substrates in 3000 rpm and annealed at 65°C for 5 minutes.

## Structure Determination through X-ray diffraction

### Single crystal X-ray crystallography

The single crystal structures of (FBA)<sub>2</sub>PbBr<sub>4</sub>, (R-FMBA)<sub>2</sub>PbBr<sub>4</sub>, and (S-FMBA)<sub>2</sub>PbBr<sub>4</sub> were obtained using Rigaku XtaLAB Synergy-S diffractometer equipped with a HyPix-6000HE Hybrid Photon Counting (HPC) detector and dual Mo and Cu microfocus sealed X-ray sources. The crystals were attached to cryoloop with Paratone-N oil. The data were collected at room temperature. The structures were solved using Olex2 software where XT

refinement package using Least Squares minimization were employed in solving and refining the structures, respectively. Table S1 summarizes the refinement details and the resulting factors. CIF files have been deposited with the CCDC: 2260472 for (R-FMBA)<sub>2</sub>PbBr<sub>4</sub>, 2260473 for (S-FMBA)<sub>2</sub>PbBr<sub>4</sub>. VESTA was used as the crystal structure visualization software for the images presented in the manuscript.

## Powder X-ray Diffraction

PXRD analysis was performed on Rigaku SmartLab powder X-Ray diffractometer with the PhotonMax high-flux 9 kW rotating anode X-ray source coupled with a 1D measurement modes. The diffraction pattern was scanned over the angular range of 3-50 degrees ( $2\theta$ ) with a step size of 0.03 at room temperature.

**Table 1.** Room temperature crystallographic data for (FBA)<sub>2</sub>PbBr<sub>4</sub>, (R-FMBA)<sub>2</sub>PbBr<sub>4</sub>, and (S-FMBA)<sub>2</sub>PbBr<sub>4</sub>.

| Compound                                | (FBA) <sub>2</sub> PbBr <sub>4</sub>                                             | (R-FMBA) <sub>2</sub> PbBr <sub>4</sub>                                          | (S-FMBA) <sub>2</sub> PbBr <sub>4</sub>                                          |
|-----------------------------------------|----------------------------------------------------------------------------------|----------------------------------------------------------------------------------|----------------------------------------------------------------------------------|
| Formula                                 | C <sub>14</sub> H <sub>18</sub> Br <sub>4</sub> F <sub>2</sub> N <sub>2</sub> Pb | C <sub>16</sub> H <sub>22</sub> Br <sub>4</sub> F <sub>2</sub> N <sub>2</sub> Pb | C <sub>16</sub> H <sub>22</sub> Br <sub>4</sub> F <sub>2</sub> N <sub>2</sub> Pb |
| Formula weight/g mol <sup>-1</sup>      | 779.13                                                                           | 807.18                                                                           | 807.18                                                                           |
| Temperature/K                           | 298.51(10)                                                                       | 296.93(10)                                                                       | 297.5(8)                                                                         |
| Crystal system                          | monoclinic                                                                       | orthorhombic                                                                     | orthorhombic                                                                     |
| Space group                             | P2 <sub>1</sub> /c (14)                                                          | P2 <sub>1</sub> 2 <sub>1</sub> 2 (19)                                            | P2 <sub>1</sub> 2 <sub>1</sub> 2 (19)                                            |
| a/Å                                     | 17.5495(2)                                                                       | 7.88037(11)                                                                      | 7.88175(4)                                                                       |
| b/Å                                     | 8.14960(10)                                                                      | 8.82621(13)                                                                      | 8.82647(6)                                                                       |
| c/Å                                     | 8.11350(10)                                                                      | 33.7831(5)                                                                       | 33.8097(18)                                                                      |
| $\alpha$ / °                            | 90                                                                               | 90                                                                               | 90                                                                               |
| $\beta$ / °                             | 99.7440(10)                                                                      | 90                                                                               | 90                                                                               |
| $\gamma$ / °                            | 90                                                                               | 90                                                                               | 90                                                                               |
| V/Å <sup>3</sup>                        | 1143.66(2)                                                                       | 2349.74(6)                                                                       | 2351.95(2)                                                                       |
| Z                                       | 2                                                                                | 4                                                                                | 4                                                                                |
| $\rho_{\text{cal}}$ /g cm <sup>-3</sup> | 2.263                                                                            | 2.282                                                                            | 2.280                                                                            |
| F(000)                                  | 712                                                                              | 1488                                                                             | 1488                                                                             |
| $2\theta$ range/°                       | 10.23 to 160.44 (0.78 Å)                                                         | 10.36 to 178.80 (0.77 Å)                                                         | 10.36 to 154.99 (0.79 Å)                                                         |
| Reflections collected                   | 31481                                                                            | 61323                                                                            | 67076                                                                            |
| Independent reflections                 | 2470                                                                             | 4976                                                                             | 4952                                                                             |
| R <sub>int</sub>                        | 0.1583                                                                           | 0.1293                                                                           | 0.0659                                                                           |
| R <sub>sigma</sub>                      | 0.0468                                                                           | 0.0344                                                                           | 0.0201                                                                           |
| Data/constraints/parameters             | 2470/0/98                                                                        | 4976/0/231                                                                       | 4952/0/230                                                                       |
| Goodness-of-fit on F <sup>2</sup>       | 1.077                                                                            | 1.104                                                                            | 1.048                                                                            |
| Final R indices $\geq 2\sigma(I)$       | R <sub>1</sub> = 0.0564, wR <sub>2</sub> = 0.1668                                | R <sub>1</sub> = 0.0359, wR <sub>2</sub> = 0.0773                                | R <sub>1</sub> = 0.0221, wR <sub>2</sub> = 0.0623                                |
| Final R indices [all data]              | R <sub>1</sub> = 0.0569, wR <sub>2</sub> = 0.1680                                | R <sub>1</sub> = 0.0383, wR <sub>2</sub> = 0.0798                                | R <sub>1</sub> = 0.0224, wR <sub>2</sub> = 0.0625                                |

## Absorption Analysis

Steady-state optical spectra of the crystals were measured at room temperature and 77K (liquid nitrogen to cool the samples) using FS5 spectrofluorometer (Edinburgh Instruments). and (S-FMBA)<sub>2</sub>PbBr<sub>4</sub> exhibit chiroptical absorption in the 275–400 nm wavelength range.
